# Supplementary material for: Helimagnon resonances in an intrinsic chiral magnonic crystal
Source: arXiv:1705.02874 ancillary file (2017-11-20)
Supplement: Supplementary file 1 [file CSO_Spinwaves_SI2.pdf]

# Supplemental Information: Helimagnon resonances in an intrinsic chiral magnonic crystal


Mathias Weiler,[1,2,*] Aisha Aqeel,[3,†] Maxim Mostovoy,[3] Andrey Leonov,[3,4] Stephan Geprägs,[1] Rudolf Gross,[1,2,5] Hans Huebl,[1,2,5] Thomas T. M. Palstra,[3,‡] and Sebastian T. B. Goennenwein[1,2,5,6,7]

[1] *Walther-Meißner-Institut, Bayerische Akademie der Wissenschaften, Garching, Germany*
[2] *Physik-Department, Technische Universität München, Garching, Germany*
[3] *Zernike Institute for Advanced Materials, University of Groningen, Groningen, The Netherlands*
[4] *Center for Chiral Science, Hiroshima University, Japan*
[5] *Nanosystems Initiative Munich, Munich, Germany*
[6] *Institut für Festkörper- und Materialphysik, Technische Universität Dresden, Dresden, Germany*
[7] *Center for Transport and Devices of Emergent Materials, Technische Universität Dresden, Dresden, Germany*



(Dated: November 2, 2017)


## DATA PROCESSING

At each value of $H_0$, a complex-valued $S_{21}$ trace was recorded as a function of frequency $f$ with the VNA. To nullify the frequency-dependent (but $H_0$ independent) background in $S_{21}(f, H_0)$ which stems from the frequency-dependent transmission through the CPW-$Cu_2OSeO_3$ hybrid and microwave cable assemblies we then calculate [1]

$$\delta S_{21}(f, H_0) \equiv \frac{S_{21}(f, H_0 + \delta H_0) - S_{21}(f, H_0 - \delta H_0)}{S_{21}(f, H_0)}\,, \tag{S1}$$

which is proportional to the difference quotient of $S_{21}(f, H_0)$ with respect to $H_0$. Division by $S_{21}(f, H_0)$ removes the effect of electrical length and losses in the CPW and microwave cables.

## EXPERIMENTALLY DETERMINED HELIMAGNON RESONANCE FREQUENCIES

Figure S1 shows the same data as Fig. 3 in the main text, with adjusted colorcode to enhance the contrast. We superimpose the resonance fields shown in Fig. 4 in the main text on the $\delta S_{21}$ data by the dotted lines. The resonance fields correspond to the lowest frequency dipolar helimagnon mode for $n = 1$ (bottom row), $n = 2$ (middle row) and $n = 3$ (top row). The resonance frequencies, $f_{\mathrm{res}}(H_0)$, shown in Fig. 4(b) in the main text are calculated from the mean of the resonance frequencies $f_{\mathrm{res}}(\pm H_0)$. Different $f_{\mathrm{res}}$ are observed for inverted $\boldsymbol{H}_0$-directions are attributed to domain formations because they are hysteretic and depend on $H_0$ sweep direction.

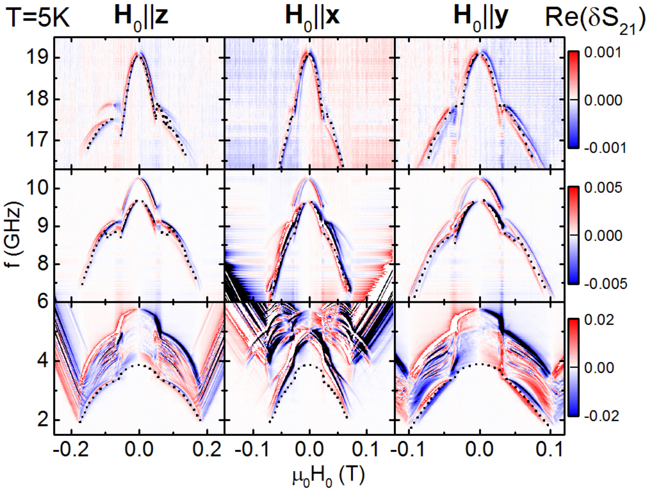


Figure S1. Same data as in Figure 3 in the main text, with adjusted colorcode to enhance contrast. The dotted lines correspond to the resonance frequencies shown in Fig. 4 in the main text.

## EXPERIMENTALLY DETERMINED HELIMAGNON RESONANCE LINEWIDTHS

The narrow linewidths that we observe for all helimagnon resonances discussed in the main text are quite remarkable, given previous reports of large damping in the ferrimagnetic phase of $Cu_2OSeO_3$ at higher temperature [2]. To estimate the helimagnon damping, we here focus on data obtained in the helical phase where the lowest number of dipolar spin-waves are observed due to the vanishing net magnetization. Figure S2 shows data recorded with $\mu_0 H_0 = 30\,\mathrm{mT}$ for $\boldsymbol{H}_0 \parallel \boldsymbol{z}$ at $T = 5\,\mathrm{K}$. Experimental data obtained for the $n = 2$ [Fig. S2(a)] and the $n = 3$ [Fig. S2(b)] mode are shown. For the $n = 1$ mode, the large number of dipolar spin waves visible in Fig. S1 prevented extraction of one individual line. The magnetic damping is given by $\alpha = \frac{1}{2}\Delta f / f_{\mathrm{res}}$, with the full width at half maximum $\Delta f$ of the magnetic resonance. We fit the $\delta S_{21}$ data to $\mathrm{Re}\left[\chi(f + \delta f) - \chi(f - \delta f)\right]$ with

$$\chi(f) = \frac{C_0}{f_{\mathrm{res}}^2 - f^2 - i f \Delta f}\,. \tag{S2}$$

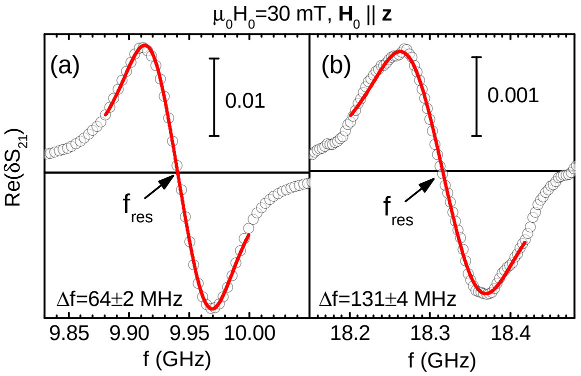


Figure S2. (a) Experimentally determined helimagnon linewidths in the helical phase for the $n = 2$ mode at $\mu_0 H_0 = 30\,\mathrm{mT}$ applied along the $\boldsymbol{z}$-direction. (b) Simultaneously recorded linewidth of the $n = 3$ mode.

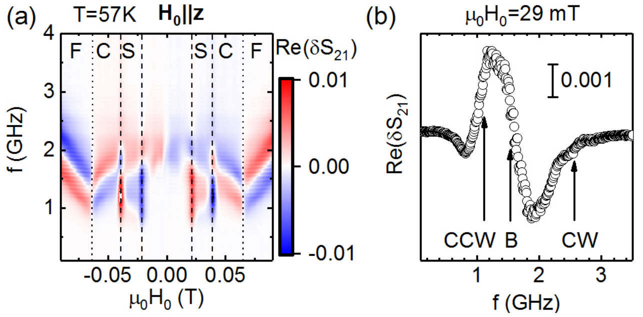


Figure S3. (a) Colorcoded $\delta S_{21}$ (see text) spectra recorded as a function of $f$ and $H_0$ at $T = 57\,\mathrm{K}$. Dashed vertical lines indicate the approximate locations of the skyrmion (S), conical (C) and ferrimagnetic (F) phase transitions. The helical (H) to C phase transition at small $|H_0|$ is not clearly visible. (b) $\delta S_{21}$ vs. $f$ for fixed $\mu_0 H_0 = 29\,\mathrm{mT}$. Three characteristic resonances of the S phase are identified: counterclockwise (CCW), breathing (B) and a weak clockwise (CW) mode.

Here, $C_0$ is the resonance amplitude, and $\delta f \propto \delta H_0$ corresponds to the effective frequency modulation of $\delta S_{21}$ caused by the non-zero magnetic field step size $\delta H_0$ as defined in Eq. (3) in the main text. $\delta f$ is treated as a fit parameter. $\Delta f$ obtained from the fitting is only independent of $\delta f$ for $\delta f \ll \Delta f$. In our measurements $\delta f \approx 30\,\mathrm{MHz}$ was actually comparable to $\Delta f$, causing a slight over-modulation and thus artificially enhanced linewidth of the helimagnon resonances. This is taken into account by fitting the data to Eq. (S2), which allows us to estimate the intrinsic $Cu_2OSeO_3$ linewidth from the data shown in Fig. S2. We extract $\Delta f = 64 \pm 2\,\mathrm{MHz}$ at $f_{\mathrm{res}} = 9.943 \pm 0.001\,\mathrm{GHz}$ for the $n = 2$ mode and $\Delta f = 131 \pm 4\,\mathrm{MHz}$ at $f_{\mathrm{res}} = 18.317 \pm 0.002\,\mathrm{GHz}$ for the $n = 3$ mode. Assuming negligible inhomogeneous broadening and identical damping for the $n = 2$ and $n = 3$ modes, both linewidths are compatible with $\alpha = 0.5\Delta f / f_{\mathrm{res}} \approx 0.003$. For the used input power of 1 mW, the driving microwave magnetic field at the CPW with a 100 µm wide center conductor is estimated to be smaller than 0.03 mT. Using $g = 2.1$, this corresponds $f = g\mu_B / h\mu_0 H = 1\,\mathrm{MHz}$, much smaller than the linewidths observed in Fig. S2, so that non-linear effects are not expected to contribute to the observed linewidths.

## SKYRMION RESONANCES

In addition to the data recorded at $T = 5\,\mathrm{K}$ that is discussed in the main text, we also performed corresponding VNA spectroscopy of the $Cu_2OSeO_3$ sample at higher temperatures. At $T = 57\,\mathrm{K}$ and with $\boldsymbol{H}_0 \parallel \boldsymbol{z}$, we record the VNA spectrum shown in Fig. S3(a). We identify phase transitions from the ferrimagnetic (F) to conical (C) phase (dotted lines) with same qualitative features as found at $T = 5\,\mathrm{K}$. The strong vertical features marked by the dashed vertical lines are attributed to the observation of skyrmion (S) to conical (C) phase transitions, with the S phase being enclosed by the vertical dashed lines. Fig. S3(b) shows a single $\delta S_{21}$ spectrum recorded at fixed $\mu_0 H_0 = 29\,\mathrm{mT}$, comparable to data shown in Refs. [2, 3]. Two strong and one weak resonances are observed that we attribute to counterclockwise (CCW), breathing (B) and clockwise (CW) modes of the skyrmion resonance as labeled in Fig. S3(b). The CCW and CW mode have a positive dispersion ($f$ increases with increasing $H_0$) and the B mode has a negative dispersion [2]. Hence, data in Fig. S3(b) features a dip-peak resonance for the CCW and CW mode and a peak-dip resonance for the B mode. Despite the good signal-to-noise ratio of the data in Fig. S3, we were not able to find evidence for higher order modes at this temperature. We attribute this to the strongly enhanced linewidth of all resonances compared to $T = 5\,\mathrm{K}$.

## MAGNON SPECTRUM FOR THE CONICAL SPIRAL

The excitation modes and magnetic susceptibilities are found from the solution of the Landau-Lifshitz-Gilbert equation,

$$\dot{\boldsymbol{m}} = -\gamma \boldsymbol{m} \times \mathcal{H} + \alpha \boldsymbol{m} \times \dot{\boldsymbol{m}}, \tag{S3}$$

where $\boldsymbol{m} = \frac{\boldsymbol{M}}{M}$ is the unit vector in the direction of the magnetization, $\boldsymbol{M}$, $\alpha$ is the damping parameter and $\mathcal{H} = -\frac{\delta E}{\delta \boldsymbol{M}}$ with the energy, $E$, given by

$$E = \int d^3x \left[\frac{\rho_s}{2}\left(\partial_i \boldsymbol{m} \cdot \partial_i \boldsymbol{m} + 2Q\boldsymbol{m} \cdot \boldsymbol{\nabla} \times \boldsymbol{m}\right) - \mu_0 \boldsymbol{M} \cdot \boldsymbol{H}\right]$$
$$-\frac{\mu_0 M^2}{8\pi} \int d^3x d^3x' \frac{[3(\boldsymbol{m}(\boldsymbol{x}) \cdot \hat{\boldsymbol{r}})(\boldsymbol{m}(\boldsymbol{x}') \cdot \hat{\boldsymbol{r}}) - \boldsymbol{m}(\boldsymbol{x}) \cdot \boldsymbol{m}(\boldsymbol{x}')]}{r^3}. \tag{S4}$$

The first three terms are, respectively, the exchange, Dzyaloshinskii-Moriya and Zeeman interactions, $\rho_s$ is the effective exchange constant and $Q$ is the length of the spiral wave vector. The last term in Eq. (S4) is the dipole-dipole interaction with $\boldsymbol{r} = \boldsymbol{x} - \boldsymbol{x}'$ and $\hat{\boldsymbol{r}} = \frac{\boldsymbol{r}}{r}$.

We first find the static spin configuration for the magnetic field, $\boldsymbol{H} = H_0\hat{\boldsymbol{z}}$, where $\hat{z}$ is the unit vector in the $z$ direction. Substitution of the spiral Ansatz,

$$\boldsymbol{m}_0 = \cos\theta\hat{\boldsymbol{z}} + \sin\theta\left(\cos(Qz)\hat{\boldsymbol{x}} + \sin(Qz)\hat{\boldsymbol{y}}\right), \quad \text{(S5)}$$

into Eq. (S3) gives $\mathcal{H} = \rho_s Q^2 \boldsymbol{m}_0$ and the expression for the conical angle,

$$\cos\theta = \frac{\mu_0 M H_0}{\rho_s Q^2 + \mu_0 N_z M^2}, \quad \text{(S6)}$$

where

$$N_z = -\frac{1}{4\pi}\int d^3x \frac{(3\hat{r}_z^2 - 1)}{r^3} \quad \text{(S7)}$$

is the demagnetization factor for the $z$ direction (we assume, for simplicity, that the sample has an ellipsoidal shape).

In the ac magnetic field $\boldsymbol{h}(t)$, $\boldsymbol{m}(\boldsymbol{x},t) = \boldsymbol{m}_0(\boldsymbol{x}) + \delta\boldsymbol{m}(\boldsymbol{x},t)$ and the linearized equation for $\delta\boldsymbol{m}$ obtained from Eq. (S3) reads

$$\delta\dot{\boldsymbol{m}} - \alpha\boldsymbol{m}_0 \times \delta\dot{\boldsymbol{m}} - [\boldsymbol{m}_0 \times \delta\boldsymbol{F}] = -\gamma\mu_0[\boldsymbol{m}_0 \times \boldsymbol{h}] \quad \text{(S8)}$$

with

$$\delta\boldsymbol{F} = D_s\left(-\triangle\delta\boldsymbol{m} + 2Q[\boldsymbol{\nabla}\times\delta\boldsymbol{m}] + Q^2\delta\boldsymbol{m}\right) - \frac{\gamma\mu_0 M}{4\pi}\int\frac{d^3x'}{r^3}\left[3\hat{\boldsymbol{r}}(\hat{\boldsymbol{r}}\cdot\delta\boldsymbol{m}(\boldsymbol{x}')) - \delta\boldsymbol{m}(\boldsymbol{x}')\right], \quad \text{(S9)}$$

$D_s = \frac{\gamma\rho_s}{M}$ being the spin stiffness.

For $\boldsymbol{h}(t) = \boldsymbol{h}_0\cos\omega t$, $\delta\boldsymbol{m} = \Re e(\boldsymbol{\xi}e^{i\omega t})$. Since $(\delta\boldsymbol{m}\cdot\boldsymbol{m}_0) = 0$,

$$\boldsymbol{\xi}(\boldsymbol{x}) = \xi_\theta(\boldsymbol{x})\boldsymbol{e}_\theta(z) + \xi_\varphi(\boldsymbol{x})\boldsymbol{e}_\varphi(z), \quad \text{(S10)}$$

where

$$\begin{aligned}\boldsymbol{e}_\theta(z) &= \frac{\partial\boldsymbol{m}_0}{\partial\theta} = (\cos\theta\cos\varphi, \cos\theta\sin\varphi, -\sin\theta),\\ \boldsymbol{e}_\varphi(z) &= \frac{1}{\sin\theta}\frac{\partial\boldsymbol{m}_0}{\partial\varphi} = (-\sin\varphi, \cos\varphi, 0)\end{aligned} \quad \text{(S11)}$$

with $\varphi = Qz$. Equation (S10) is the transformation to the co-rotating spin frame.

For the spatially uniform amplitude of the ac magnetic field, $\boldsymbol{h}_0$, $\xi_\theta$ and $\xi_\varphi$ only depend on $z$ and can be written as the Fourier series:

$$\begin{cases}\xi_\theta(z) = \sum_n \xi_\theta^{(n)}e^{iQnz},\\ \xi_\varphi(z) = \sum_n \xi_\varphi^{(n)}e^{iQnz}.\end{cases} \quad \text{(S12)}$$

For the spiral wave length, $\frac{2\pi}{Q}$ much smaller than the linear dimensions of the sample, the demagnetization field is different for zero and nonzero Fourier harmonics:

$$-\frac{1}{4\pi}\int\frac{d^3x'}{r^3}(3\hat{r}_i\hat{r}_j - \delta_{ij})e^{iQnz'} = \begin{cases}\delta_{ij}N_i, & \text{for } n = 0,\\ \delta_{iz}\delta_{jz}e^{iQnz}, & \text{for } n \neq 0,\end{cases} \quad \text{(S13)}$$

where $\delta_{ij}$ is the Kronecker symbol and $N_i$ is the demagnetization factor for the $i$-th direction of the ellipsoid. The $n = 0$ mode is the translational mode of the spiral and the $n \neq 0$ modes are the precessional modes. Equations for the $n = \pm 1$ modes are different from those for other precessional modes because only the $n = \pm 1$ modes induce a spatially uniform oscillating magnetization in the lab frame. The resulting demagnetization field couples equations for these modes, which can be written in the form

$$\begin{aligned}&-i\Omega\xi_\theta^+ + iy\cos\theta\xi_\theta^- + (1 - i\alpha\Omega + y)\xi_\varphi^+ = \gamma_y,\\ &-i\Omega\xi_\theta^- + ix\cos\theta\xi_\theta^+ + (1 - i\alpha\Omega + x)\xi_\varphi^- = i\gamma_x,\\ &-i\Omega\xi_\varphi^+ + ix\cos\theta\xi_\varphi^- - (1 - i\alpha\Omega + (1+\chi)\sin^2\theta + x\cos^2\theta)\xi_\vartheta^+ = -\gamma_x\cos\theta,\\ &-i\Omega\xi_\varphi^- + iy\cos\theta\xi_\varphi^+ - (1 - i\alpha\Omega + (1+\chi)\sin^2\theta + y\cos^2\theta)\xi_\vartheta^- = i\gamma_y\cos\theta,\end{aligned} \quad \text{(S14)}$$

where $\xi_\theta^\pm = \frac{1}{2}(\xi_\theta^{(+1)} \pm \xi_\theta^{(-1)})$ and $\xi_\varphi^\pm = \frac{1}{2}(\xi_\varphi^{(+1)} \pm \xi_\varphi^{(-1)})$, $\Omega = \frac{\omega}{D_sQ^2}$ is the dimensionless frequency, $\chi = \frac{\gamma\mu_0 M}{D_sQ^2}$ is the strength of the dipole-dipole interactions, $x = \frac{\chi N_x}{2}$, $y = \frac{\chi N_y}{2}$ and $\gamma_x = \frac{\chi h_x}{2M}$, $\gamma_y = \frac{\chi h_y}{2M}$ are the dimensionless transverse components of the ac magnetic field.

The spatially uniform part of the oscillating magnetization, $\langle\boldsymbol{\xi}\rangle$, is given by

$$\begin{aligned}\langle\xi_x\rangle &= \xi_\theta^+\cos\theta - i\xi_\varphi^-,\\ \langle\xi_y\rangle &= i\xi_\theta^-\cos\theta - \xi_\varphi^+,\end{aligned} \quad \text{(S15)}$$

which allows to find magnetic susceptibilities from Eq. (S14), e.g.,

$$\chi_{xx} = \frac{M\langle\xi_x\rangle}{h_x} = \frac{\chi}{2\gamma_x}(\xi_\theta^+\cos\theta - i\xi_\varphi^-). \quad \text{(S16)}$$

The four eigenfrequencies, at which the susceptibilities have poles (at zero damping) are given by

$$\Omega_\pm^2 = \frac{b \pm \sqrt{b^2 - 4c}}{2}, \quad \text{(S17)}$$

where

$$\begin{aligned}b &= \cos^2\theta(x + y + 4xy) + (2 + x + y)(1 + (1+\chi)\sin^2\theta),\\ c &= [x\cos^2\theta + (1 + x)(1 + (1+\chi)\sin^2\theta)]\\ &\quad\times[y\cos^2\theta + (1 + y)(1 + (1+\chi)\sin^2\theta)].\end{aligned} \quad \text{(S18)}$$

At the second critical field, $H_{c2}$, $\theta = 0$, $\Omega_+ = (1+2x)(1+2y)$ and $\Omega_- = 1$. Using $\mu_0 H_{c2} M = \rho_s Q^2 + \mu_0 M^2 N_z$, following from Eq. (S6), and $N_x + N_y + N_z = 1$, one can show that the expression for $\Omega_+$ coincides with the Kittel formula for the ferromagnetic resonance frequency at this value of the magnetic field,

$$\omega_{\rm FMR}^2 = (\gamma\mu_0)^2 (H_{c2} - (N_z - N_x)M)(H_{c2} - (N_z - N_y)M). \quad \text{(S19)}$$

The mode with the frequency $\Omega_-$ is decoupled from the ac magnetic field: the peak corresponding to this eigenfrequency vanishes as $H$ approaches $H_{c2}$ from below and in the collinear ferromagnetic state ($H > H_{c2}$) only the ferromagnetic resonance remains.

The magnetic excitation modes with $n \neq \pm 1$ are decoupled from each other and from the spatially uniform ac magnetic field:

$$\begin{cases} -i\Omega(\xi_\theta^{(n)} + \alpha\xi_\varphi^{(n)}) = -n^2 \xi_\varphi^{(n)} \\ -i\Omega(\xi_\varphi^{(n)} - \alpha\xi_\theta^{(n)}) = (n^2 + (1+\chi)\sin^2\theta)\alpha\xi_\theta^{(n)}. \end{cases} \quad \text{(S20)}$$

The eigenfrequency of the $n$-th mode is then given by

$$\Omega_n^2 = n^2(n^2 + (1+\chi)\sin^2\theta). \quad \text{(S21)}$$

With $\rho_s Q^2 = DQ = \frac{MB_{c2}}{1+N_z\chi}$ the last equation gives Eq. (1) in the main text. The fitting of the experimentally determined resonance frequencies (Figure 4 in the main text) uses $\Omega_-$ from Eq. (S17) for $n = 1$ and $\Omega_n$ from Eq. (S21) for $n = 2$ and $n = 3$.

## MAGNETOSTATIC MODES

The large number of peaks in the vicinity of the $n = \pm 1$ modes (see Fig. 4a in the main text) can be ascribed to magnetostatic modes [4, 5]. Rather than calculating frequencies of all individual magnetostatic modes, we estimate their lowest and highest frequency using the idea of Clogston *et al.* [6], which we apply to the conical spiral state. Consider a magnetic excitation, which in the co-rotating spin frame has the wave length much larger than the period of the spiral but much smaller than the linear sample dimension, $L$. In this case Eq. (S12) is replaced with

$$\begin{cases} \xi_\theta(z) = e^{i\boldsymbol{k}\cdot\boldsymbol{x}} \sum_n \xi_\theta^{(n)} e^{iQnz}, \\ \xi_\varphi(z) = e^{i\boldsymbol{k}\cdot\boldsymbol{x}} \sum_n \xi_\varphi^{(n)} e^{iQnz}, \end{cases} \quad \text{(S22)}$$

where $\boldsymbol{k}$ is the wave vector in the co-rotating frame, such that $L^{-1} \ll k \ll Q$. In this regime, the spectrum of magnetic excitations depends on the direction of the wave vector $\boldsymbol{k}$ with respect to the applied magnetic field, $\boldsymbol{H}_0 \parallel \boldsymbol{Q}$, but is practically independent of the absolute value, $k$.

The demagnetization field for such excitations is obtained using

$$-\frac{1}{4\pi}\int \frac{d^3x'}{r^3}(3\hat{r}_i\hat{r}_j - \delta_{ij}) e^{i(n\boldsymbol{Q}+\boldsymbol{k})\cdot\boldsymbol{x}'} = \\ = e^{i(n\boldsymbol{Q}+\boldsymbol{k})\cdot\boldsymbol{x}} \begin{cases} \hat{k}_i\hat{k}_j, & \text{for } n = 0, \\ \delta_{iz}\delta_{jz}, & \text{for } n \neq 0, \end{cases} \quad \text{(S23)}$$

(cf. Eq. (S13)) and the coupled equations of motion for the $n = \pm 1$ modes have the form,

$$\begin{aligned} -i\Omega\xi_\theta^+ + \xi_\varphi^+ + \tfrac{1}{2}\chi\hat{k}_y(\hat{\boldsymbol{k}}\cdot\boldsymbol{\xi}^{(0)}) &= 0, \\ -i\Omega\xi_\theta^- + \xi_\varphi^- + \tfrac{i}{2}\chi\hat{k}_x(\hat{\boldsymbol{k}}\cdot\boldsymbol{\xi}^{(0)}) &= 0, \\ -i\Omega\xi_\varphi^+ + (1 + (1+\chi)\sin^2\theta)\xi_\theta^+ - \tfrac{1}{2}\chi\hat{k}_x(\hat{\boldsymbol{k}}\cdot\boldsymbol{\xi}^{(0)}) &= 0, \\ -i\Omega\xi_\varphi^- + (1 + (1+\chi)\sin^2\theta)\xi_\theta^- + \tfrac{i}{2}\chi\hat{k}_y(\hat{\boldsymbol{k}}\cdot\boldsymbol{\xi}^{(0)}) &= 0, \end{aligned} \quad \text{(S24)}$$

where $\boldsymbol{\xi}^{(0)}$ is the amplitude of the oscillating magnetization with the wave vector $\boldsymbol{k}$ in the lab frame:

$$(\boldsymbol{k}\cdot\boldsymbol{\xi}^{(0)}) = \hat{k}_x(\cos\theta\xi_\theta^+ - i\xi_\varphi^-) + i\hat{k}_y(\cos\theta\xi_\theta^- - i\xi_\varphi^+). \quad \text{(S25)}$$

Solving Eq. (S24), we obtain the frequency that depends on the direction of $\boldsymbol{k}$:

$$\Omega^2 = 1 + (1+\chi)\sin^2\theta + \frac{1}{2}(2 + \chi\sin^2\theta)\sin^2\alpha_{\boldsymbol{k}}, \quad \text{(S26)}$$

where $\alpha_{\boldsymbol{k}}$ is the angle between $\boldsymbol{k}$ and $\boldsymbol{H}_0$. The minimum and maximum frequencies of the 'magnetostatic band' are given by

$$\begin{aligned} \Omega_{\rm min} &= \sqrt{1 + (1+\chi)\sin^2\theta}, \\ \Omega_{\rm max} &= \sqrt{1 + \chi + (1 + \chi + \frac{1}{2}\chi^2)\sin^2\theta}. \end{aligned} \quad \text{(S27)}$$

Their magnetic field dependence is shown in Fig. S4 (dotted lines), where we also plot $\Omega_+$ and $\Omega_-$ (red and blue lines, respectively) obtained from Eq. (S17). As visible from Fig. S4, the $\Omega_-$ mode is close to the minimum frequency of the magnetostatic band. We hence approximately identify the $\Omega_-$ mode as the lowest frequency $n = 1$ mode in the main text.

At $H_{c2}$, Eq. (S26) gives the expression obtained earlier for the ferromagnetic state [6]:

$$\omega = \gamma\mu_0\sqrt{(H_{c2} - N_z M)(H_{c2} - N_z M + M\sin^2\alpha_{\boldsymbol{k}})}. \quad \text{(S28)}$$

## EFFECT OF MAGNETIC ANISOTROPIES

The excitation of the $|n| > 1$ modes with a uniform magnetic field becomes possible when magnetic anisotropies are taken into account. Consider the fourth-order

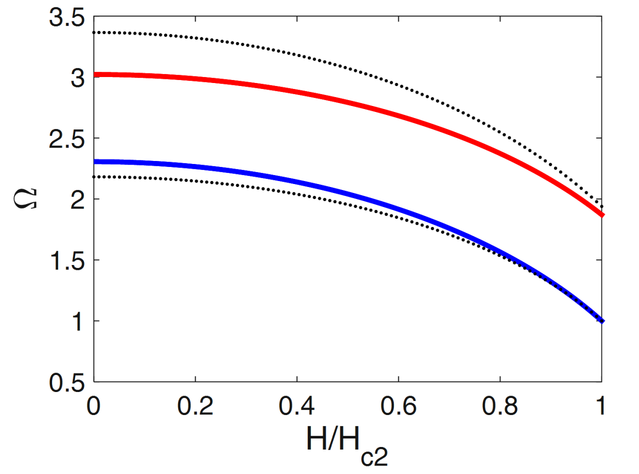


Figure S4. Maximal and minimal frequencies of the magnetostatic band (dotted lines) together with the frequencies of the modes excited by the homogenious ac magnetic field $\Omega_+$ (red line) and $\Omega_-$ (blue line) (see Eq. (S17)) as a function of the applied magnetic field in the conical spiral phase. The calculation was done for $\chi = 2.76$, $N_x = 0.665$, $N_y = 0.085$, and $N_z = 0.250$.

anisotropy energy,

$$E_{\rm ani} = K(m_a^4 + m_b^4 + m_c^4), \tag{S29}$$

allowed by cubic symmetry, where the indices $a, b$ and $c$ label projections of $\boldsymbol{m}$ on the corresponding cubic axes.

For the $x$, $y$ and $z$ axes oriented as shown in Fig. 2 in the main text,

$$E_{\rm ani} = K\left[\frac{1}{2} + m_z^2 - \frac{7}{6}m_z^4 - \frac{2\sqrt{2}}{3}m_z(m_x^3 - 3m_x m_y^2)\right], \tag{S30}$$

which can be expressed in terms of the polar angles, $\theta$ and $\varphi$ ($(m_x, m_y, m_z) = (\sin\theta\cos\varphi, \sin\theta\sin\varphi, \cos\theta)$):

$$E_{\rm ani} = K\left(\frac{1}{2} + \cos^2\theta - \frac{7}{6}\cos^4\theta - \frac{2\sqrt{2}}{3}\cos\theta\sin^3\theta\cos 3\varphi\right). \tag{S31}$$

The $\cos 3\varphi = \cos 3Qz$ dependence of the anisotropy energy gives rise to a non-uniform spin rotation in the conical spiral. More importantly, it couples the magnetic excitation with the wave vector $q$ to excitations with the wave vectors $q \pm 3Q$. Thus the $n = \mp 1$ mode becomes coupled to the $n = \pm 2$, which makes the higher-order modes "visible" in the magnetic absorption spectrum.

## ELECTRIC FIELD EXCITATION OF MAGNETIC MODES

$P2_13$ symmetry of $Cu_2OSeO_3$ allows for the following form of the magnetoelectric coupling between the electric polarization, $\boldsymbol{P}$, and the magnetization vector, $\boldsymbol{m}$:

$$E_{\rm me} = -g_{\rm me}\int dV\,(E_a m_b m_c + E_b m_c m_a + E_c m_a m_b). \tag{S32}$$

For the $x$, $y$ and $z$ axes oriented as shown in Fig. 2 in the main text,

$$E_{\rm me} = -\frac{g_{\rm me}}{\sqrt{3}}\int dV\left[E_x\left(\frac{(m_y^2 - m_x^2)}{\sqrt{2}} - m_x m_z\right)\right.$$
$$\left. + E_y(\sqrt{2}m_x - m_z) + E_z\left(m_z^2 - \frac{(m_x^2 + m_y^2)}{2}\right)\right]. \tag{S33}$$

One can then define an 'effective ac field', $\boldsymbol{h}_{\rm eff}$, induced by the ac electric field, $\boldsymbol{e}$:

$$\boldsymbol{h}_{\rm eff} = -\frac{1}{\mu_0 M}\frac{\partial E_{\rm me}}{\delta \boldsymbol{m}}. \tag{S34}$$

The effective ac field in the co-rotating spin frame is obtained by projecting $\boldsymbol{h}_{\rm eff}$ on the unit vectors $\boldsymbol{e}_\theta$ and $\boldsymbol{e}_\varphi$:

$$(\boldsymbol{h}_{\rm eff}\cdot\boldsymbol{e}_\varphi) = \frac{g_{\rm me}}{\sqrt{3}\mu_0 M}\left[\sin\theta(E_x\sin 2\varphi + E_y\cos 2\varphi)\right.$$
$$\left. + \cos\theta(E_x\sin\varphi - E_y\cos\varphi)\right],$$
$$(\boldsymbol{h}_{\rm eff}\cdot\boldsymbol{e}_\theta) = \frac{g_{\rm me}}{\sqrt{3}\mu_0 M}\left[\frac{\sin 2\theta}{\sqrt{2}}(E_x\cos 2\varphi - E_y\sin 2\varphi)\right.$$
$$\left. + \cos 2\theta(E_x\cos\varphi + E_y\sin\varphi) + 3E_z\sin 2\theta\right], \tag{S35}$$

with $\varphi = Qz$, showing that the ac electric field excites both $n = \pm 1$ and $n = \pm 2$ harmonics with comparable intensities (unless the cone angle $\theta$ is close to 0 or $\frac{\pi}{2}$).

The ratio of the amplitudes of the electric and magnetic excitations of the $n = \pm 1$ harmonics can be estimated as

$$r = \frac{h_{eff}}{h} \sim \frac{g_{\rm me}}{\sqrt{3}\mu_0 M}\frac{e}{h}. \tag{S36}$$

The ratio of the amplitudes of the ac electric and magnetic fields, $\frac{e}{h} \sim \frac{\mu_0 c}{\sqrt{\epsilon_\infty}}$, where $\epsilon_\infty$ is the background dielectric constant and $c$ is the speed of light, which gives

$$r \sim \frac{g_{\rm me}V_0 c}{8\sqrt{3}\mu_{\rm B}\sqrt{\epsilon_\infty}}, \tag{S37}$$

where $V_0$ is the unit cell volume and we took into account that the magnetic moment of the unit cell is $\sim 8\mu_B$.

The values of the magnetoelectric coupling constant, which one can deduce from literature, vary widely. Using $g_{\rm me} = 32\,\mu{\rm C}\cdot{\rm m}^{-2}$ (obtained from $P_{[001]} = 16\,\mu{\rm C}\cdot{\rm m}^{-2}$ in the ferrimagnetic state induced by $\boldsymbol{H} \parallel [110]$) and $\epsilon_\infty = 8$ (see Ref. [7]), we obtain $r \sim 3\cdot 10^{-2}$. On the other hand, $g_{\rm me} = 2.4\,\mu{\rm C}\cdot{\rm m}^{-2}$ (obtained from $P_{[111]} = 1.4\,\mu{\rm C}\cdot{\rm m}^{-2}$ in the ferrimagnetic state induced by $\boldsymbol{H} \parallel [111]$) and

$\epsilon_\infty = 12.5$ (see Ref. [8]) gives $r \sim 2 \cdot 10^{-3}$. In any case, since the ratio of the spectral weights of the electric and magnetic absorption peaks is $r^2$, one can conclude that the magnetoelectric coupling in $Cu_2OSeO_3$ is too weak to explain the observed excitation of the higher harmonics.

* mathias.weiler@wmi.badw.de
† present address: University of Regensburg, Regensburg, Germany
‡ present address: The University of Twente, Enschede, The Netherlands

[1] H. Maier-Flaig, S. T. B. Goennenwein, R. Ohshima, M. Shiraishi, R. Gross, H. Huebl, and M. Weiler, arXiv , 1705.05694 (2017).
[2] T. Schwarze, J. Waizner, M. Garst, A. Bauer, I. Stasinopoulos, H. Berger, C. Pfleiderer, and D. Grundler, Nat. Mater. **14**, 478 (2015).
[3] Y. Onose, Y. Okamura, S. Seki, S. Ishiwata, and Y. Tokura, Phys. Rev. Lett. **109**, 037603 (2012).
[4] L. R. Walker, Phys. Rev. **105**, 390 (1957).
[5] L. R. Walker, J. Appl. Phys. **29**, 318 (1958).
[6] A. M. Clogston, H. Suhl, L. R. Walker, and P. W. Anderson, J. Phys. Chem. Solids **1**, 129 (1956).
[7] M. Mochizuki and S. Seki, J. Phys.: Condens. Matter **27**, 503001 (2015).
[8] E. Ruff, P. Lunkenheimer, A. Loidl, H. Berger, and S. Krohns, Sci. Rep. **5**, 15025 (2015).
